# Supplementary material for: Decoherence and fidelity enhancement during shuttling of entangled spin qubits
Source: arXiv:2506.19671 source file (2025-06-24)
Supplement: Supplementary file 1 [file SpinShuttling3-PRB-Lett-SI-Fin.pdf]

# Supplemental Material

# "Decoherence and fidelity enhancement during shuttling of entangled spin qubits"

Yu-Ning Zhang, Aleksandr S. Mokeev, and Viatcheslav V. Dobrovitski

*QuTech and Kavli Institute of Nanoscience, Delft University of Technology, PO Box 5046, 2600 GA Delft, The Netherlands*

## CONTENTS

I. Zeeman Hamiltonian of the shuttled spin 2

II. Dephasing during shuttling of two entangled qubits 6

III. Dephasing factor for two entangled qubits shuttled through Ornstein-Uhlenbeck random sheet 8
A. Autocorrelation terms 9
B. Cross-correlation terms 12

IV. Dephasing factor for two entangled qubits shuttled through Gaussian “pink” sheet with $1/f$ noise spectrum in time and exponential correlation decay in space 16
A. Covariance integrals for pink sheet 17
B. Asymptotic expansion 21

References 22

## I. ZEEMAN HAMILTONIAN OF THE SHUTTLED SPIN

The Zeeman energy of the shuttled electron spin is affected by the shape of its wavepacket $\rho(\vec{r}; x_c)$ and the position of its center $x_c$. In most devices, a nominally uniform quantizing magnetic field $B_Q \sim 0.1$–$1$ T is applied to the system. However, the effective $g$-factor of the electron slightly varies in space due to random variations in the material properties, such that the Zeeman energy of the electron spin varies in space:

$$H_{B_Q}(x_c) = S_z \int d^3r\, g(\vec{r})\, \mu_B\, B_Q\, \rho(\vec{r}; x_c), \tag{1}$$

where we assume (i) that the quantization axis does not vary in space (e.g. because the $g$-tensor is practically isotropic, as in Si-based systems, or because its principal axes have the same directions everythwere in the sample), and (ii) that the variations of the $g$-factor in space are not too large.

Besides, if randomly located nuclear spins are present in the system, then the position-dependent random hyperfine field $B_{\mathrm{hf}}$ should be taken into account; this can be done within the Kohn–Luttinger theory [1]. The hyperfine coupling between the nuclear spin $I_n$ located

at the position $\vec{r}_n$ and the spin of an electron occupying the atomic orbital near the bottom of the conduction band (or the hole near the top of the valence band) [1] of the atom at the position $\vec{r}_a$ has a form [2]

$$H_{\mathrm{hf},n} = \vec{S} \cdot \mathcal{D}(\vec{r}_a - \vec{r}_n) \cdot \vec{I}_n, \tag{2}$$

where we combined all relevant terms (local contact and dipolar contributions, as well as the long-range dipolar couplings) in a single tensor $\mathcal{D}$. Since the field $B_Q$ is strong, and the quantization axis is assumed to be directed along the $z$-axis everythwere, we can neglect the non-secular terms (proportional to $S_x$ and $S_y$) in the rotating-frame approximation [2, 3]. We also take into account that the electron wavepacket $\rho(\vec{r}; x_c)$ is spead over many atoms and interacts with many nuclei, such that the summation over both $\vec{r}_a$ (weighted with the density $\rho(\vec{r}; x_c)$) and $\vec{r}_n$ should be performed, giving

$$H_{\mathrm{hf}}(x_c) = S_z \int d^3r\, \rho(\vec{r}; x_c) \sum_{\vec{r}_n} \vec{D}(\vec{r} - \vec{r}_n) \cdot \vec{I}_n, \tag{3}$$

where $\vec{D}$ is a shorthand notation for the part of the tensor $\mathcal{D}$ corresponding to the $S_z$ component, i.e. $D_\alpha \equiv \mathcal{D}_{z,\alpha}$, with $\alpha = x, y, z$. Now, we take into account that the operators of the nuclear spins $\vec{I}_n$ change in time, as a result of the coupling between different nuclear spins (mostly dipolar interactions, but also electron-mediated transfer coupling), as well as possible quadrupolar interactions, etc. The complex dynamics of this bath of nuclear spins can be approximated as random, and the hyperfine coupling Hamiltonian is simplified to

$$H_{\mathrm{hf}}(x_c, t) = g_s \mu_B S_z \int d^3r\, \rho(\vec{r}; x_c)\, B_{\mathrm{hf}}(\vec{r}, t), \tag{4}$$

where $g_s \approx 2.002$ is the spin $g$-factor of a free electron, $\mu_B$ is Bohr's magneton, and $B_{\mathrm{hf}}(\vec{r}, t)$ is an effective hyperfine magnetic field, randomly changing in both space and time.

Under ideal conditions, for a perfect running-wave confining potential and in the absense of any inhomogeneities in the shuttling channel, the shape of the wavepacket would stay constant during shuttling, and the density profile would have a perfect automodel form $\rho(\vec{r}; x_c) = \rho_0(x - x_c, y, z)$. In reality, random variation of the material properties along the shuttling channel slightly change the shape of the confining potential, such that the the density distribution $\rho(x, y, z; x_c)$ reflects these changes and slightly varies as the wavepacket center $x_c$ moves. Moreover, there is a large number of charged defects present in real systems, such as the charge traps, which can randomly trap and release electrons, or where

the trapped charge can randomly jump between two nearby positions. These events also affect the electrostatic potential felt by the shuttled electron, and lead to small random displacements and distortions of the wavepacket. Therefore, the electron density $\rho(x, y, z; x_c)$ becomes explicitly dependent on both $x_c$ and time,

$$\rho(\vec{r}, t; x_c) = \rho_0(x - x_c, y, z) + \Delta\rho(x, y, z, t; x_c). \tag{5}$$

As seen from Eqs. (1) and (4) above, such variations lead to the randomly varying in space and time Hamiltonian of the form

$$\tilde{H}_Z(x_c, t) = \mu_B S_z \int d^3r \left[g(\vec{r}) B_Q + g_s B_{\text{hf}}(\vec{r}, t)\right] \rho(\vec{r}, t; x_c), \tag{6}$$

which can be re-written in a familiar form

$$\tilde{H}_Z(x_c, t) = g_0 \mu_B \left[B_0(x_c) + \tilde{B}(x_c, t)\right] S_z \tag{7}$$

where $g_0$ is a nominal $g$-factor of the electron in the semiconducting channel (the appropriately averaged value of $g(\vec{r})$, see below), while $B_0(x_c, t)$ and $\tilde{B}(x_c, t)$ represent, respectively, the deterministic and the random part of the effective magnetic field; more precise meaning of these terms is discussed below.

The confining potential created by the clavier gates slightly differs from an ideal traveling wave due to the finite gate pitch: the potential periodically changes its shape, and so does the wavepacket of the shuttled electron. If the phase shift between the adjacent pairs of the gates is small enough, then these changes are small [4, 5] and can be neglected. However, if needed, the periodic changes in the shape of the wavepacket can also be taken into account with minor modifications of the approach outlined in this work. In that case, we should take into account that the deterministic part of the wavepacket now has the form $\rho_0(\vec{r}, t)$, and upon substitution in Eq. (6), we obtain the Zeeman Hamiltonian

$$\tilde{H}_Z(x_c, t) = g_0 \mu_B \left[B_0(x_c, t) + \tilde{B}(x_c, t)\right] S_z, \tag{8}$$

where the notations are the same as in Eq. (8), except that now the deterministic part $B_0(x_c, t)$ of the effective field explicitly depends on time. Upon shuttling along the given trajectory $x_c(t)$ during the time interval $0 \geq t \geq t_0$, the deterministic and the random fields acting on the electron spin become equal to $B_0(t) = B_0(x_c(t), t)$ and $\mathrm{B}(t) = \tilde{B}(x_c(t), t)$,

respectively, such that the wavefunction of the electron spin during shuttling acquires the deterministic and the random phases

$$\alpha(t_0) = \int_0^{t_0} B_0(t)dt, \text{ and } \phi(t_0) = \int_0^{t_0} \mathrm{B}(t)dt. \tag{9}$$

respectively. The rest of the analysis can be performed in the same way as outlined in the text, except that the statistical properties (mean and covariance) of the random field $\mathrm{B}(t)$ now may reflect the periodic changes in the wavepacket envelope $\rho_0(\vec{r}, t)$. We do not study such modifications here, firstly, they would be small for sufficiently smooth shuttling, and, secondly, they would depend on the specific experimental settings.

It may be also helpful to explicate a subtle feature of the Hamiltonian $\tilde{H}_Z(x_c, t)$ in Eq. (8). The field $\tilde{B}(x_c, t)$ randomly varies from one experiment to another, such that its value cannot be predicted in advance, while the value of $B_0(x_c)$ can be predicted, at least in principle. Therefore, the delineation between these parts depends on the specific experimental setting. For instance, if we consider a device where the quenched disorder in $g(\vec{r})$ leads to appearance of an effective field $B_{\text{q.d.}}(\vec{r}) = g(\vec{r})\mu_B B_Q$ that does not vary with time, then $B_{\text{q.d.}}$ should be viewed as deterministic: while the profile $B_{\text{q.d.}}(\vec{r})$ is not known in advance, but it can be measured once (at least, in principle) and used later to reliably predict its influence on the shuttled qubits. But if we are studying a large batch of similar devices with different profiles $B_{\text{q.d.}}(\vec{r})$, or the same device where $B_{\text{q.d.}}(\vec{r})$ fluctuates slowly but randomly (such that the previous measurements cannot be re-used later) then this field should be considered as random, a part of $\tilde{B}(x_c, t)$. In a similar way, if the trajectories $x_c(t)$ of the qubits slightly fluctuate from one experimental shot to another, then the deterministic quantity $B_0(x_c)$ gives rise to a random contribution to the magnetic field acting on the spin. In this work, we consider all qubits trajectories $x_c(t)$ and the field $B_0(x_c)$ as deterministic, we also assume that the ideal-case wavepacket $\rho_0(x - x_c, y, z)$ does not explicitly depend on time and that the average hyperfine field is zero, such that the condition

$$g_0 B_0(x_c) = \int d^3r\, g(\vec{r}) B_Q\, \rho_0(x - x_c, y, z), \tag{10}$$

see Eqs. (6) and (8), determines the quantities $g_0$ and $B_0$.

Finally, we note that the approach used in this work is most useful in the situations where the total shuttling distance $L$ is noticeably larger than the characteristic width of the envelope $\rho(\vec{r}, t; x_c)$. Otherwise, it may be more advantageous to explicitly determine the

shape of $\rho(\vec{r}, t; x_c)$ and work directly with Eq. (6), although modeling of the noise $\tilde{B}(x,t)$ as a random Gaussian sheet would still be helpful. The approach presented here can also be extended to include other important features of the actual devices, e.g. to take into account that the the effective magnetic field acting on the shuttled spin is a vector $\vec{B}(x_c, t)$, such that the spin decoherence includes random rotations around the $x$ and $y$ axes. It may be also extended to include into consideration the spin-orbit interaction and excitations to the excited valley states and higher orbitals of the shuttling potential [4–8]. Such extensions fall out of the scope of this work.

## II. DEPHASING DURING SHUTTLING OF TWO ENTANGLED QUBITS

The most straightforward approach to qubit shuttling is to encode the state of a qubit $a|0\rangle + b|1\rangle$ in a state of a single electron spin as $|\psi_0\rangle = a|\uparrow\rangle + b|\downarrow\rangle$ and shuttle the electron. In the course of shuttling during time interval $0 \le t \le t_f$, due to joint action of the deterministic $B_0(t)$ and the random $\mathrm{B}(t)$ magnetic fields, the spin acquires additional deterministic $\alpha = \int_0^{t_f} B_0(t)\, dt$ and random $\phi = \int_0^{t_f} \mathrm{B}(t)\, dt$ phases, such that the spin state becomes $|\psi_\Theta\rangle = a|\uparrow\rangle + b\exp\{i\Theta\}\,|\downarrow\rangle$. The deterministic phase $\alpha$ can be taken into account during post-processing, and can be set to zero. The random phase factor $\exp\{i\phi\}$, averaged over the noise $\mathrm{B}(t)$, decreases the off-diagonal elements $\langle 0|\rho|1\rangle$ and $\langle 1|\rho|0\rangle$ of the qubit density matrix $\rho$ by a factor $W_1 = \mathbb{E}\,\exp\{-i\phi\}$ (the diagonal elements of $\rho$ remain unaffected by the noise along the $z$-axis). As a result, the qubit is decohered, and fidelity of the qubit shuttling process is equal to $F_1 = (1 + W_1)/2$, where the subscript “1” denotes encoding of a qubit with a single electron spin.

The dephasing factor $W_1$ for a single-qubit shuttling remains finite even if the noise $\tilde{B}(x_c, t)$ is quasi-static in time, with $\kappa_t \to 0$. This happens because the random field $\mathrm{B}(t)$ acquires nontrivial dependence on time due to variation of the noise in space, through the time variation of $x_c(t)$. An alternative analyzed in this work is to encode the state of the qubit in a decoherence-free subspace of a logical qubit [9–11], formed by the singlet and triplet states of two electron spins. These spins are shuttled with some delay one after another, similar to e.g. Ref. 12, where the shuttling of the singlet state was studied experimentally. In order to substantiate this proposal, it is crucial to analyze its performance under realistic circumstances, and identify the range of parameters where such an encoding

would be beneficial.

Assume that we have a state of a spin qubit $a|\uparrow\rangle + b|\downarrow\rangle$ that is to be shuttled from one quantum dot to another. We use an ancilla spin, located e.g. in an adjacent dot and prepared in a state $|\uparrow\rangle$, such that the two-spin wavefunction is a product $[a|\uparrow_1\rangle + b|\downarrow_1\rangle]\,|\uparrow_2\rangle$, where the subscripts 1 and 2 denote the states of the qubit and the ancilla, respectively. Then we apply a CNOT gate with the qubit as a control and ancilla as a target, turning the two-spin state into

$$|\psi_0\rangle = a\,|\uparrow_1\downarrow_2\rangle + b\,|\downarrow_1\uparrow_2\rangle = a'\,|\Psi^+\rangle + b'\,|\Psi^-\rangle, \tag{11}$$

with $a' = (a+b)/\sqrt{2}$ and $b' = (a-b)/\sqrt{2}$, thus encoding the original qubit state into a linear combination of the singlet $|\Psi^-\rangle = (|\uparrow_1\downarrow_2\rangle - |\downarrow_1\uparrow_2\rangle)/\sqrt{2}$ and the triplet $|\Psi^+\rangle = \frac{1}{\sqrt{2}}[|\uparrow_1\downarrow_2\rangle + |\downarrow_1\uparrow_2\rangle]$. After the encoding, the two spins are sequentially shuttled to the destination, where the decoding is done with another CNOT gate, turning the states $|\uparrow_1\downarrow_2\rangle$ and $|\downarrow_1\uparrow_2\rangle$ back into the qubit states $|\uparrow\rangle$ and $|\downarrow\rangle$.

We assume that the first electron is loaded into the shuttling channel at $t = 0$, while the second electron is waiting in the original quantum dot, at $x = 0$. After the delay $T_0$, the second electron starts shuttling. During the whole process, both electrons are confined in the minima of the moving potential, moving as tightly localized wavepackets with centers at $x = x_{c1}$ and $x = x_{c2}$. The minimal delay is determined by the period of the confining potential, i.e. by the pitch of the clavier gates and by the frequency of the oscillating confining potential. After the first electron reaches the destination quantum dot ($x = L$) at time $t = T_1$, it is assumed to stay there until the second electron is transported to the right end of the shuttling channel at $t = t_f = T_2$.

During this two-spin shuttling, the state of the qubit is modified due to the action of the noises $\mathrm{B}_1(t)$ and $\mathrm{B}_2(t)$ acting on the first and the second spin, respectively, and the random phases acquired by the spins turn the original qubit state into $|\psi_\phi\rangle = a\,|0\rangle + b\exp\{i\phi_2\}\,|1\rangle$, where $\phi_2 = \int_0^{t_f} (\mathrm{B}_1(t) - \mathrm{B}_2(t))\,dt$ because of the opposite $z$-components of the spins in both basis states $|\uparrow_1\downarrow_2\rangle$ and $|\downarrow_1\uparrow_2\rangle$. Averaging over the noise reduces the off-diagonal elements $\langle 0|\rho|1\rangle$ and $\langle 1|\rho|0\rangle$ of the qubit density matrix $\rho$ by a factor $W_2 = \mathbb{E}\exp\{-i\phi_2\}$, and the fidelity of the qubit state after shuttling becomes equal to $F_2 = (1 + W_2)/2$, where the subscript "2" denotes encoding of a qubit with two electron spins.

In order to calculate the dephasing factor $W_2$, we assume that the shuttling of each spin occurs with the same constant velocity $v$ between the same initial ($x_c = 0$) and final ($x_c = L$)

points. Thus, the trajectories of the two spins are

$$x_{c1}(t) = \begin{cases} vt, & 0 < t \le T_1 \\ L, & T_1 < t < T_2 \end{cases}, \qquad x_{c2}(t) = \begin{cases} 0, & 0 < t \le T_0 \\ v(t - T_0), & T_0 < t < T_2 \end{cases}. \tag{12}$$

Depending on the shuttling velocity $v$ and the delay $T_0$, the second spin starts shuttling before or after the first spin reaches the final point, i.e. $T_0 \le T_1$ and $T_0 > T_1$, respectively.

As discussed above, the random processes $\mathrm{B}_1(t)$ and $\mathrm{B}_2(t)$, defined by the trajectories $x_{c1}(t)$ and $x_{c2}(t)$ on the Gaussian random sheet $\tilde{B}(x_c, t)$, are Gaussian, and their difference $\delta\mathrm{B}(t) = \mathrm{B}_1(t) - \mathrm{B}_2(t)$ is also Gaussian, such that

$$W_2 = \mathbb{E}\, e^{-i\phi_2} = \exp\{-\chi_2\}, \qquad \chi_2 = \frac{1}{2} \int_0^{t_0} \int_0^{t_0} K_{\delta\mathrm{B}}(t_1, t_2)\, dt_1 dt_2, \tag{13}$$

where covariance of the process $\delta\mathrm{B}(t)$ is

$$\begin{aligned} K_{\delta\mathrm{B}}(t_1, t_2) &= \mathbb{E}\left[ (\mathrm{B}_1(t_1) - \mathrm{B}_2(t_1))\, (\mathrm{B}_1(t_2) - \mathrm{B}_1(t_2)) \right] \\ &= \mathbb{E}\left[\mathrm{B}_1(t_1)\mathrm{B}_1(t_2)\right] + \mathbb{E}\left[\mathrm{B}_2(t_1)\mathrm{B}_2(t_2)\right] - \mathbb{E}\left[\mathrm{B}_2(t_1)\mathrm{B}_1(t_2)\right] - \mathbb{E}\left[\mathrm{B}_1(t_1)\mathrm{B}_2(t_2)\right] \end{aligned} \tag{14}$$

The first two terms above represent the autocorrelations of $\mathrm{B}_1(t)$ and $\mathrm{B}_2(t)$, while the last two terms represent the cross-correlation between them, which are non-trivial because both processes are derived from the same underlying random sheet $\tilde{B}(x_c, t)$.

## III. DEPHASING FACTOR FOR TWO ENTANGLED QUBITS SHUTTLED THROUGH ORNSTEIN-UHLENBECK RANDOM SHEET

Statistical properties of the random processes $\mathrm{B}_{1,2}(t)$ are determined by the underlying space- and time-dependent noise $\tilde{B}(x_c, t)$. This noise, being indexed by two continuous variables $x_c$ and $t$, is not a conventional random process indexed indexed by one variable. In this work we treat the noise $\tilde{B}(x_c, t)$ using the mathematical concept of Gaussian random sheet [13–15], which generalizes the idea of a Gaussian random process. Mathematical details of our approach are presented elsewhere [16]. For this work, it is important only to mention the following. Firstly, all statistical properties of the Gaussian random sheet $\tilde{B}(x_c, t)$ are defined by its mean, which we set to zero (non-zero mean can be included in the deterministic phase $\alpha$), and the two-point covariance function $K(x_c, t; x'_c, t')$. Secondly,

for any realistic spin trajectory $x_c(t)$, the corresponding random process $\mathrm{B}(t)$ is a Gaussian random process with zero mean and the covariance function $K_{\mathrm{B}}(t,t') = K(x_c(t),t;x'_c(t'),t')$. It is important to point out that Gaussianity is the only property that is reliably inherited by the processes $\mathrm{B}_{1,2}(t)$ from the underlying sheet $\tilde{B}(x_c,t)$. Other properties, often assumed in modeling of physical systems, are not that simple. For instance, if the spin moves along a non-trivial trajectory through a *stationary* Gaussian sheet, the noise acting on the spin is in general *non-stationary*. Discussion of the Markov property is even more difficult, even correctly defining Markov random sheet is a highly non-trivial mathematical task [15, 16]. Fortunately, Gaussian property by itself is sufficient for modeling of a broad variety of realistic noises.

A particularly illustrative and non-trivial, but, at the same time, reasonably simple model, is Ornstein-Uhlenbeck (OU) sheet with the covariance function

$$K_{\mathrm{OU}}(x_c,t;x'_c,t') = \sigma_{\mathrm{B}}^2 \, \exp\{-\kappa_x|x_c - x'_c| - \kappa_t|t-t'|\}. \tag{15}$$

This model describes stationary Gaussian noise with the correlations which exponentially decay in both space and time, as has been observed in many semiconductor system [4, 17–22], with the correlation length $\lambda_c = 1/\kappa_x$ and the correlation time $\tau_c = 1/\kappa_t$.

Once the covariance of the underlying Gaussian sheet is specified, the dephasing factor can be calculated as described above, by Eqs. (13) and (14). The details of the calculation are presented below; the calculations were performed mostly using the package Mathematica 13.3 [23].

### A. Autocorrelation terms

First, we calculate the autocorrelation terms of the random processes $\mathrm{B}_1(t)$ and $\mathrm{B}_2(t)$, which describe decoherence of individual spins.

We start by evaluating the contribution produced by the autocorrelation of the field $\mathrm{B}_1(t)$ acting on the first spin, calculating the integral

$$I_{11} = \exp\left\{-\int_0^T \mathrm{d}t_1 \int_0^T \mathrm{d}t_2 \, K_{\mathrm{B}1}(t_1,t_2)\right\}, \tag{16}$$

where $K_{\mathrm{B}1}(t_1,t_2) = \mathbb{E}\left[\mathrm{B}_1(t_1)\mathrm{B}_1(t_2)\right]$ is the covariance function of the field $\mathrm{B}_1(t)$ (the first term in Eq. 14), and therefore $K_{\mathrm{B}1}(t_1,t_2) = K_{OU}(x_{c1}(t_1),t_1;x_{c1}(t_2),t_2)$. This function depends on

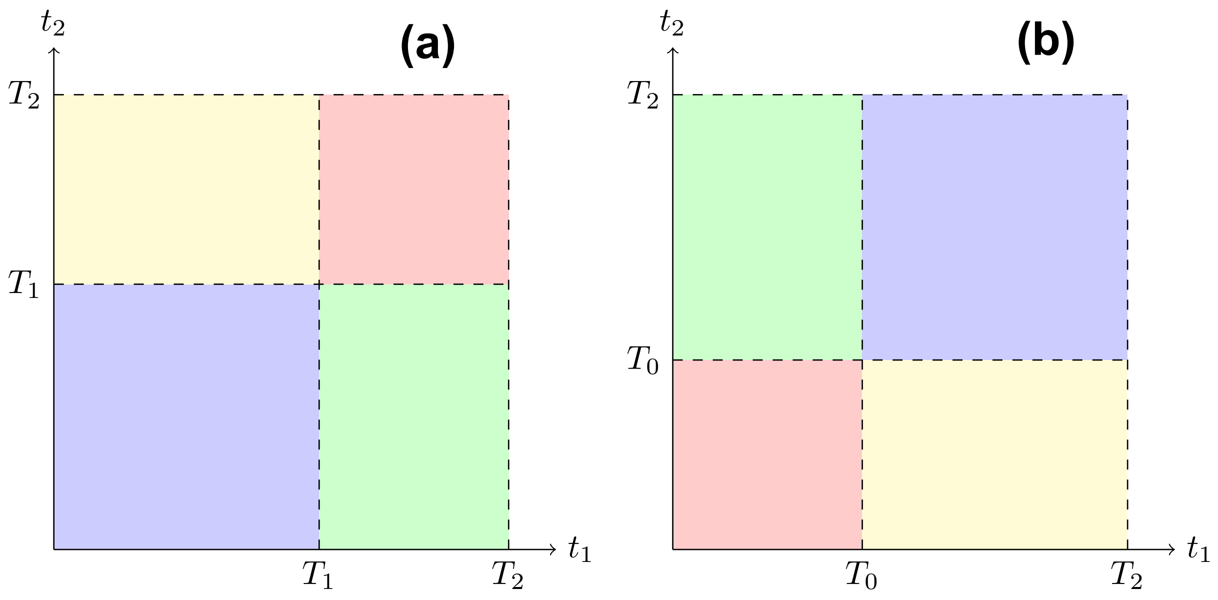


FIG. 1. Division of the integration area into different regions when calculating the contributions of the autocorrelation terms. **(a)**: Integration of $K_{\mathrm{B1}}(t_1, t_2) = \mathbb{E}[B_1(t_1)B_1(t_2)]$. **(b)**: Integration of $K_{\mathrm{B2}}(t_1, t_2) = \mathbb{E}[B_2(t_1)B_2(t_2)]$.

the difference $x_{c1}(t_1) - x_{c1}(t_2)$, which is equal to

$$x_{c1}(t_1) - x_{c1}(t_2) = \begin{cases} v(t_1 - t_2) & \text{in } \mathbf{B}, \\ L - vt_2 & \text{in } \mathbf{G}, \\ vt_1 - L & \text{in } \mathbf{Y}, \\ 0 & \text{in } \mathbf{R}, \end{cases} \tag{17}$$

where we divided the whole integration area into four regions as shown in Fig. 1a, shading each region with the corresponding color:

$$\begin{aligned} \mathbf{B} \text{ (blue)}: &\quad t_1 \in [0, T_1],\ t_2 \in [0, T_1], \\ \mathbf{G} \text{ (green)}: &\quad t_1 \in [T_1, T_2],\ t_2 \in [0, T_1], \\ \mathbf{Y} \text{ (yellow)}: &\quad t_1 \in [0, T_1],\ t_2 \in [T_1, T_2], \\ \mathbf{R} \text{ (red)}: &\quad t_1 \in [T_1, T_2],\ t_2 \in [T_1, T_2]. \end{aligned} \tag{18}$$

Evaluating the integral $I_{11}$ in each region, we obtain:

$$\begin{aligned}
\mathbf{B:}\ P_1 =& \int_0^{T_1} \mathrm{d}t_1 \int_0^{T_1} \mathrm{d}t_2 \, \exp\{-(\kappa_t + \kappa_x L/T_1)|t_1 - t_2|\} \\
&= 2T_1^2 \cdot \frac{e^{-L\kappa_x - T_1\kappa_t} + L\kappa_x + T_1\kappa_t - 1}{(L\kappa_x + T_1\kappa_t)^2} && (19) \\
\mathbf{R:}\ P_2 =& \int_{T_1}^{T_2} \mathrm{d}t_1 \int_{T_1}^{T_2} \mathrm{d}t_2 \, \exp\{-\kappa_t|t_1 - t_2|\} \\
&= \frac{2}{\kappa_t^2} \left[\kappa_t T_0 + e^{-\kappa_t T_0} - 1\right] && (20) \\
\mathbf{G:}\ P_3 =& \\
& \int_{T_1}^{T_2} \mathrm{d}t_1 \int_0^{T_1} \mathrm{d}t_2 \, \exp\{-\kappa_t(t_1 - t_2) - \kappa_x L(1 - t_2/T_1)\} \\
&= \frac{T_1 \left(1 - e^{-T_0\kappa_t}\right)\left(1 - e^{-L\kappa_x - T_1\kappa_t}\right)}{\kappa_t \left(L\kappa_x + T_1\kappa_t\right)} && (21) \\
\mathbf{Y:}\ P_4 =& \\
& \int_0^{T_1} \mathrm{d}t_1 \int_{T_1}^{T_2} \mathrm{d}t_2 \, \exp\{-\kappa_t(t_2 - t_1) - \kappa_x L(1 - t_1/T_1)\} \\
&= \frac{T_1 \left(1 - e^{-T_0\kappa_t}\right)\left(1 - e^{-L\kappa_x - T_1\kappa_t}\right)}{\kappa_t \left(L\kappa_x + T_1\kappa_t\right)} && (22)
\end{aligned}$$

Note that the correlation function $K_{\mathrm{B1}}(t_1, t_2)$ is symmetric with respect to interchange of the variables $t_1$ and $t_2$, such that the integrals $P_3$ and $P_4$ are equal.

In the same way, we calculate the terms involving the autocorrelations of the field $\mathrm{B}_2(t)$ acting on the second spin, described by the covariance function $K_{\mathrm{B2}}(t_1, t_2)$:

$$I_{22} = \exp\left\{-\int_0^T \mathrm{d}t_1 \int_0^T \mathrm{d}t_2 \, K_{\mathrm{B2}}(t_1, t_2)\right\}. \tag{23}$$

The function $K_{\mathrm{B2}}(t_1, t_2)$ is determined by the trajectory $x_{c2}(t)$ of the second spin, and involves the difference $x_{c2}(t_1) - x_{c2}(t_2)$. Again, we divide the integration area into four regions as shown in Fig. 1b, but now the color coding is different:

$$\begin{aligned}
\mathbf{B}\ (\text{blue}): &\quad t_1 \in [T_0, T_2],\ t_2 \in [T_0, T_2], && (24) \\
\mathbf{G}\ (\text{green}): &\quad t_1 \in [0, T_0],\ t_2 \in [T_0, T_2], \\
\mathbf{Y}\ (\text{yellow}): &\quad t_1 \in [T_0, T_2],\ t_2 \in [0, T_0], \\
\mathbf{R}\ (\text{red}): &\quad t_1 \in [0, T_0],\ t_2 \in [0, T_0].
\end{aligned}$$

With this color coding, the quantity $x_{c2}(t_1) - x_{c2}(t_2)$ is equal to

$$x_{c2}(t_1) - x_{c2}(t_2) = \begin{cases} v(t_1 - t_2) & \text{in } \mathbf{B}, \\ v(T_0 - t_2) & \text{in } \mathbf{G}, \\ v(t_1 - T_0) & \text{in } \mathbf{Y}, \\ 0 & \text{in } \mathbf{R}. \end{cases} \tag{25}$$

The reason for different encoding becomes clear when we compare Eqs. (25) and (17), take into account that, firstly, $T_2 - T_0 = T_1$ (both spins are shuttled with the same velocity, so the shuttling times are equal) and secondly, that the covariance function of the underlying OU sheet $K_{OU}(x, t; x', t')$ is translationally invariant in time and space. As a result, it is not difficult to see that the integrals $I_{22}$ and $I_{11}$ over the regions denoted by the same letters/colors are equal, and we have

$$I_{11} = I_{22} = P_1 + P_2 + P_3 + P_4. \tag{26}$$

### B. Cross-correlation terms

Next, we evaluate the contribution from the cross-correlations between the fields $\mathrm{B}_1(t)$ and $\mathrm{B}_2(t)$ (the term $\mathbb{E}\left[\mathrm{B}_1(t_1)\mathrm{B}_2(t_2)\right]$ in Eq. 14), calculating the integral

$$I_{12} = \exp\left\{ -\int_0^T \mathrm{d}t_1 \int_0^T \mathrm{d}t_2 \, K_{\mathrm{B}12}(t_1, t_2) \right\}, \tag{27}$$

where the cross-covariance function $K_{\mathrm{B}12}(t_1, t_2) = K_{OU}[t_1, x_{c1}(t_1); t_2, x_{c2}(t_2)]$. Since both spins are shuttled with the same velocity, and the underlying OU sheet is stationary, the contribution coming from the other cross-correlation term, $\mathbb{E}\left[\mathrm{B}_2(t_1)\mathrm{B}_1(t_2)\right]$ in Eq. (14), is also equal to $I_{12}$.

As before, we subdivide the whole integration area in four regions, see Fig. 2,

$$\begin{aligned} \mathbf{B}\ \text{(blue)}: &\quad t_1 \in [0, T_1],\ t_2 \in [0, T_0] \\ \mathbf{G}\ \text{(green)}: &\quad t_1 \in [T_1, T_2],\ t_2 \in [0, T_0] \\ \mathbf{Y}\ \text{(yellow)}: &\quad t_1 \in [0, T_1],\ t_2 \in [T_0, T_2] \\ \mathbf{R}\ \text{(red)}: &\quad t_1 \in [T_1, T_2],\ t_2 \in [T_0, T_2] \end{aligned} \tag{28}$$

in accordance with the quantity $x_1(t_1) - x_2(t_2)$, which is equal to

$$x_{c1}(t_1) - x_{c2}(t_2) = \begin{cases} vt_1 & \text{in } \mathbf{B}, \\ L & \text{in } \mathbf{G}, \\ v(t_1 - t_2 + T_0) & \text{in } \mathbf{Y}, \\ L - v(t_2 - T_0) & \text{in } \mathbf{R}. \end{cases} \tag{29}$$

This quantity is positive in the regions **B**, **G**, and **R**, but in the region **Y**, the sign of $x_1(t_1) - x_2(t_2)$ changes as the line $t_2 = t_1 + T_0$ is crossed (shown as dashed red line in Fig. 2). Besides, the quantity $t_1 - t_2$ changes the sign when crossing the line $t_1 = t_2$ (solid red line in Fig. 2). Thus, the whole integration area is naturally divided into several parts, schematically shown in Fig. 2, according to the form of the covariance function $K_{OU}[t_1, x_{c1}(t_1); t_2, x_{c2}(t_2)]$, and these parts have different shape, depending on whether the delay time $T_0$ is larger or smaller than the single-spin shuttling time $T_1$.

Before performing integration, it is worthwhile to notice that in the case $T_0 > T_1$ the

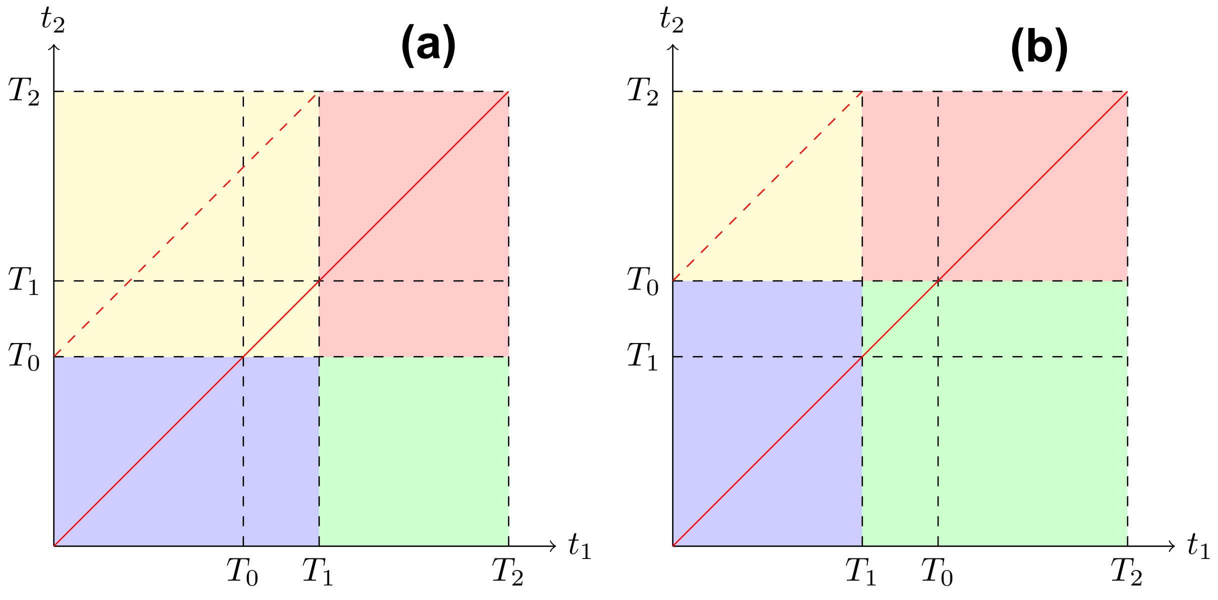


FIG. 2. Division of the integration area into different regions when calculating the contributions of the cross-correlation terms. **(a)**: The case when $T_1 > T_0$. **(b)**: The case when $T_1 < T_0$.

integral over the region **R** has the form

$$\int_{T_1}^{T_2}\int_{T_1}^{0}\exp\left\{-\kappa_t\left|T_2-t_2'-t_1\right|-\frac{\kappa_x L t_2'}{T_1}\right\}\mathrm{d}t_2'\mathrm{d}t_1,$$
$$=\int_{T_0}^{0}\int_{T_1}^{0}\exp\left\{-\kappa_t\left|t_1'-t_2'\right|-\frac{\kappa_x L t_2'}{T_1}\right\}\mathrm{d}t_2'\mathrm{d}t_1,$$

and is equal to the integral over the region **B** (the second line of the equation above); here we used the change of variables $t_2'=T_1+T_0-t_2=T_2-t_2$ and $t_1'=T_2-t_1$. In a similar manner, one can see that the integrals over **B** and **R** are also equal in the case $T_0<T_1$.

Performing the calculations for the case $T_0>T_1$, we obtain

$$\mathbf{G:}\quad C_1'=\int_{T_1}^{T_2}\int_{0}^{T_0}\exp\{-\kappa_t|t_1-t_2|-\kappa_x L\}\mathrm{d}t_2\mathrm{d}t_1 \tag{30}$$
$$=\frac{e^{-L\kappa_x}}{\kappa_t^2}\left[2(T_0-T_1)\kappa_t-e^{-T_1\kappa_t}+e^{(T_1-T_0)\kappa_t}-e^{(T_0-T_2)\kappa_t}+e^{-T_2\kappa_t}\right]$$
$$\mathbf{B:}\quad C_2'=\int_{0}^{T_1}\int_{0}^{T_0}\exp\left\{-\kappa_t\left|t_1-t_2\right|-\frac{\kappa_x L t_1}{T_1}\right\}\mathrm{d}t_2\mathrm{d}t_1 \tag{31}$$
$$=\frac{T_1\left(e^{T_1\kappa_t}-e^{T_0\kappa_t}\right)e^{-L\kappa_x-(T_0+T_1)\kappa_t}\left(e^{L\kappa_x}-e^{T_1\kappa_t}\right)}{\kappa_t\left(T_1\kappa_t-L\kappa_x\right)}+$$
$$+\frac{T_1}{\kappa_t}\left(\frac{e^{-T_1\kappa_t}-e^{-L\kappa_x}}{T_1\kappa_t-L\kappa_x}+\frac{e^{-L\kappa_x-T_1\kappa_t}-1}{L\kappa_x+T_1\kappa_t}+\frac{2-2e^{-L\kappa_x}}{L\kappa_x}\right)$$
$$\mathbf{Y:}\quad C_3'=\int_{0}^{T_1}\int_{T_0}^{T_2}\exp\left\{-\kappa_t\left(t_2-t_1\right)+\frac{\kappa_x L}{T_1}\left|t_1-t_2+T_0\right|\right\}\mathrm{d}t_2\mathrm{d}t_1 \tag{32}$$
$$=\frac{T_1^2e^{-T_0\kappa_t}\left(e^{-L\kappa_x-T_1\kappa_t}+L\kappa_x+T_1\kappa_t-1\right)}{\left(L\kappa_x+T_1\kappa_t\right)^2}+\frac{T_1^2e^{-T_0\kappa_t}\left(e^{T_1\kappa_t-L\kappa_x}+L\kappa_x-T_1\kappa_t-1\right)}{\left(T_1\kappa_t-L\kappa_x\right)^2}$$
$$\mathbf{R:}\quad C_4'=C_2'. \tag{33}$$

In the opposite case, when $T_0 < T_1$, we have

$$\textbf{G:}\quad C_1'' = \frac{1}{\kappa_t^2}\left(e^{T_0\kappa_t} - 1\right)^2 e^{-L\kappa_x - ((T_0+T_1)\kappa_t)} \tag{34}$$

$$\textbf{B:}\quad C_2'' = \frac{T_1}{\kappa_t}\Bigg\{\frac{-e^{(T_0-T_1)\kappa_t - L\kappa_x} + e^{-L\kappa_x - T_1\kappa_t} + e^{-\frac{LT_0\kappa_x}{T_1}} - 1}{L\kappa_x + T_1\kappa_t} + \frac{1 - e^{-\frac{LT_0\kappa_x}{T_1}}}{L\kappa_x} + \tag{35}$$

$$+\frac{T_1\kappa_t\left(1 - e^{-\frac{LT_0\kappa_x}{T_1}}\right) + L\kappa_x\left(e^{-T_0\kappa_t} - 1\right)}{L\kappa_x\left(T_1\kappa_t - L\kappa_x\right)}\Bigg\}$$

$$\textbf{Y:}\quad C_3'' = \tag{36}$$

$$T_1^2\Bigg\{\frac{e^{-T_0\left(\frac{L\kappa_x}{T_1}+\kappa_t\right)}\left(e^{T_0\kappa_t}\left[L\kappa_x(T_0 - T_1)/T_1 + (T_1 - T_0)\,\kappa_t + 1\right] - e^{\frac{LT_0\kappa_x}{T_1}}\left(-L\kappa_x + T_1\kappa_t + 1\right)\right)}{\left(T_1\kappa_t - L\kappa_x\right)^2} +$$

$$\frac{e^{-T_0\kappa_t}\left(e^{-L\kappa_x - T_1\kappa_t} + L\kappa_x + T_1\kappa_t - 1\right) + e^{(T_0-T_1)\kappa_t - L\kappa_x} + e^{-\frac{LT_0\kappa_x}{T_1}}\left[(T_1 - T_0)(L\kappa_x/T_1 + \kappa_t) - 1\right]}{\left(L\kappa_x + T_1\kappa_t\right)^2}\Bigg\}$$

$$\textbf{R:}\quad C_4'' = C_2'' \tag{37}$$

Introducing the dimensionless quantities

$$\eta = \kappa_t T_1, \quad \tau = \kappa_t T_0, \quad \gamma = \kappa_x L, \tag{38}$$

which denote the dimensionless shuttling time, shuttling length, and the delay, respectively, we can re-express the result in a more compact form:

$$\chi_2 = (\sigma_{\mathrm{B}}/\kappa_t)^2\left[\sum_{j=1}^{4} P_j - \sum_{j=1}^{4} C_j\right], \tag{39}$$

where the quantities

$$\begin{aligned} P_1 &= 2\,\eta^2\frac{e^{-\eta-\gamma} + \eta + \gamma - 1}{(\eta+\gamma)^2}, \\ P_2 &= 2(\tau + e^{-\tau} - 1), \\ P_3 &= P_4 = \eta\frac{(1 - e^{-\tau})\,(1 - e^{-\eta-\gamma})}{\eta+\gamma}, \end{aligned} \tag{40}$$

come from the autocorrelations of $\mathrm{B}_1(t)$ and $\mathrm{B}_2(t)$, while $C_j$ describe the cross-correlation terms, and have different form for $T_0 > T_1$ and $T_0 \le T_1$. In the former case ($T_0 > T_1$), $C_j = C_j'$, where

$$\begin{aligned} C_1' &= \mathrm{e}^{-\eta-\gamma-\tau} - 2\mathrm{e}^{-\gamma}(\eta - \tau) + \mathrm{e}^{\eta-\gamma-\tau} - 2\mathrm{e}^{-\eta-\gamma} \\ C_3' &= \eta^2\mathrm{e}^{-\tau}\left[\frac{\mathrm{e}^{-\eta-\gamma} + \eta + \gamma - 1}{(\eta+\gamma)^2} + \frac{\mathrm{e}^{-(\gamma-\eta)} + \gamma - \eta - 1}{(\gamma-\eta)^2}\right] \\ C_2' &= C_4' = \eta\left[\frac{2(1 - \mathrm{e}^{-\gamma})}{\gamma} - \frac{\mathrm{e}^{-\tau}(1 - \mathrm{e}^{\eta-\gamma})}{\gamma-\eta} - \frac{1 - \mathrm{e}^{-\eta-\gamma}}{\eta+\gamma}\right], \end{aligned} \tag{41}$$

while in the latter case, $T_0 \leq T_1$, the quantities $C_j = C_j''$, where

$$C_1'' = (\mathrm{e}^{\tau} - 1)^2 \, \mathrm{e}^{-\gamma-\eta-\tau} \tag{42}$$

$$C_3'' = \eta^2 \Bigg\{ \frac{\mathrm{e}^{-\tau\gamma/\eta}\left[\eta - \gamma - \tau(1-\gamma/\eta) + 1\right] - \mathrm{e}^{-\tau}\left(\eta - \gamma + 1\right)}{(\eta-\gamma)^2}$$
$$+ \frac{\mathrm{e}^{-\tau}\left(\mathrm{e}^{-\gamma-\eta} + \gamma + \eta - 1\right) + \mathrm{e}^{\tau-\eta-\gamma} + \mathrm{e}^{-\frac{\tau\gamma}{\eta}}\left[\eta + \gamma - \tau(1+\gamma/\eta) - 1\right]}{(\eta+\gamma)^2} \Bigg\}$$

$$C_2'' = C_4'' = \eta \Bigg\{ \frac{\eta}{\gamma}\left(\frac{1}{\eta+\gamma} + \frac{1}{\eta-\gamma}\right)\left(1 - \mathrm{e}^{-\frac{\gamma\tau}{\eta}}\right) - (1 - \mathrm{e}^{-\tau})\left[\frac{1}{\eta-\gamma} + \frac{\mathrm{e}^{-\eta-\gamma+\tau}}{\eta+\gamma}\right] \Bigg\}.$$

The term $P_1$ characterizes the phase accumulation of the first spin during its travel, while $P_2$ represents the effect of the delay $T_0$, and has the same form as dephasing under the action of OU noise. The terms $P_3$ and $P_4$ correspond to the autocorrelations of the noise during the delay ($0 < t < T_0$) and during travel of the second spin ($T_0 < t < T_1 + T_0$). The cross-correlation terms $C_j$ have similar meaning, but more complicated form.

## IV. DEPHASING FACTOR FOR TWO ENTANGLED QUBITS SHUTTLED THROUGH GAUSSIAN "PINK" SHEET WITH $1/f$ NOISE SPECTRUM IN TIME AND EXPONENTIAL CORRELATION DECAY IN SPACE

The model of Gaussian random sheet is extremely flexible and is capable of describing a broad variety of realistic noises. Here we demonstrate its application to analysis of the charge noise with $1/f$ spectrum in time and exponentially decaying correlations in space. The action of $1/f$ charge noise on the qubit has been studied in a broad range of semiconductor quantum computing platforms [4, 17–20, 24–31]. This noise is often Gaussian, and is naturally modeled as a stationary Gaussian sheet with the covariance

$$K_{\mathrm{p}}(x_c, t; x_c', t') = \sigma_{\mathrm{B}}^2 \, \exp\{-\kappa_x |x_c - x_c'|\} \, \mathcal{T}(t - t'), \tag{43}$$

where $\mathcal{T}(t-t')$ corresponds to a time covariance function of a stationary random process whose spectral power is $\mathcal{S}(\omega) \propto 1/\omega$ in a frequency range $\omega_1 \ll \omega \ll \omega_2$. The low- and high-frequency cutoffs $\omega_1$ and $\omega_2$ are needed to ensure that the total spectral power is finite, such that the covariance function $\mathcal{T}(t-t')$ approaches 1 in the short-time limit $t \to t'$ (the most basic property ensuring sanity of the model) and decays reasonably fast in the long-time limit $|t - t'| \to \infty$. This model corresponds, for instance, to a situation where a large number of randomly switching two-level fluctuators act on the qubit with comparable strengths, and the switching times of the fluctuators are log-uniformly distributed between $\omega_1$ and $\omega_2$

[31, 32], as it happens e.g. when the fluctuators switch their state via thermoactivated jumps over the energy barrier of the height $E$, and the barrier heights are uniformly distributed between the values $E_1$ and $E_2$. The power spectal density of such a noise has the form

$$\mathcal{S}(\omega) = \frac{\sigma_B^2}{\Delta\pi|\omega|}\left[\tan^{-1}\left(\frac{|\omega|}{\omega_1}\right) - \tan^{-1}\left(\frac{|\omega|}{\omega_2}\right)\right] \propto \frac{1}{|\omega|}, \quad \text{for } \omega_1 \leq \omega \leq \omega_2, \tag{44}$$

where $\Delta = \ln(\omega_2/\omega_1)$.

The corresponding time correlation function for pink sheet is the Fourier transform of that spectral density (up to the factor $\sigma_B^2$, already explicitly inculded in Eq. 43), and has the form

$$\mathcal{T}(t-t') = \frac{1}{\Delta}\left[\mathrm{Ei}(-\omega_2|t-t'|) - \mathrm{Ei}(-\omega_1|t-t'|)\right], \tag{45}$$

where the normalization factor $\Delta$ ensures that $\mathcal{T}(0) = 1$; here $\mathrm{Ei}(x)$ is the exponential integral function.

$$\mathrm{Ei}(x) = \mathcal{P}\int_{-\infty}^{x} \frac{e^t}{t}\,\mathrm{d}t, \quad \mathrm{Ei}(-x) = -\int_{x}^{\infty} \frac{e^{-t}}{t}\,\mathrm{d}t, \quad x \in \mathbb{R} \wedge x > 0, \tag{46}$$

where $\mathcal{P}$ denotes the principal value of the integral.

Note that this correlation function can also be obtained as an integral over infinitely many OU processes with the correlation decay rates $r$ having log-uniform distribution $P(r) = 1/(r\,\Delta)$ with sharp cutoffs at $\omega_1$ and $\omega_2$, i.e.

$$\mathcal{T}(t-t') = \int_{\omega_1}^{\omega_2} dr\, P(r)\exp\{-r|t-t'|\} \tag{47}$$

This is a consequence of the fact that random telegraph process (i.e., the noise produced by a two-level fluctuator) has the same correlation function $C(t)$ as OU process, namely $C(t) \propto \exp\{-r|t|\}$. In the Gaussian regime, when the number of fluctuators or the number of OU processes goes to infinity (with all other parameters, including $\omega_1$ and $\omega_2$, staying finite, see [33]), summation over both kinds of random processes produces the same Gaussian $1/f$ noise.

### A. Covariance integrals for pink sheet

The dephasing factor for sequential shuttling of the ST qubit through pink-sheet noise is calculated in the same manner as for OU sheet, by dividing the integral into auto-correlation and cross-correlation parts. We adopt the same notations $P_1, P_2, P_3, P_4$ and $C_1, C_2, C_3, C_4$

from the previous section for the integrals over auto-correlation and cross-correlation terms. The only difference is that the covariance function of these integrals will be replaced by the corresponding covariance functon $\mathcal{T}(t-t')$ of pink sheet.

However, special properties of the $1/f$ noise (and, correspondingly, of pink sheet) require some modifications. In particular, the cutoff parameters $\omega_1$ and $\omega_2$ correspond to the lowest and the highest frequency scales (or, equivalently, the longest and the shortest time scales) of the relevant experimental system. To describe the physically relevant situation, one should consider the case when $\omega_1 \to 0$ and $\omega_2 \to \infty$. However, logarithmic corrections with respect to the parameter $\omega_1$ often enter the final answer [31, 33–35]. Therefore, in the calculations below we keep the cutoffs finite, and analyze the limits $\omega_1 \to 0$ and $\omega_2 \to \infty$ later, in Section IV B.

Also, we introduce the normalized shuttling velocity $u_p = \kappa_x v$ and the normalized delay time $\tau_p = u_p T_0$ when analyzing the shuttling through pink sheet. This normalization and the notations differ from the case of OU sheet, where the dimensionless shuttling speed and the delay time were defined as $u = \kappa_x v/\kappa_t$ and $\tau = \kappa_t T_0$. The reason is, again, the special properties of $1/f$ noise. In contrast with OU sheet, where the temporal fluctuations have a clearly defined timescale $\tau_c$, pink random sheet with its $1/f$ noise power spectrum does not have such a single well-defined timescale.

The correlation integrals for pink sheet are cumbersome but not challenging, and can be effectively evaluated using modern computational algebraic software [23]; alternatively, one can use the integral representation Eq. (47) to evaluate the integrals, reusing the results for OU random sheet given in Section III above. The results are presented below.

$$P_1 = 2\int_0^{T_1}\int_0^{t_1} \tilde{\mathcal{T}}(t_1-t_2)\exp\left(-u_p(t_1-t_2)\right)dt_2 dt_1 \\ = 2T_1^2\Big[\Theta_{P_1}(u_pT_1,\omega_2T_1) - \Theta_{P_1}(u_pT_1,\omega_1T_1)\Big], \tag{48}$$

where we use a shorthand notation $\tilde{\mathcal{T}} = \mathcal{T}\cdot\Delta$ and define the function

$$\Theta_{P1}(x,y) = \frac{e^{-x}}{x^2}\mathrm{Ei}(-y) - \frac{1-e^{-(x+y)}}{x(x+y)} + \frac{x-1}{x^2}\left[\mathrm{Ei}(-x-y) - \ln\left(\frac{x+y}{y}\right)\right]. \tag{49}$$

Note that the integral $P_1$, being an autocorrelation function of the noise acting on a single shuttled spin, also gives the dephasing factor for the single-spin shuttled through pink sheet, which is shown in Fig. 4(b) of the main text.

Furthermore,

$$
\begin{aligned}
P_2 &= 2\int_0^{T_0}\int_0^{t_1}\tilde{\mathcal{T}}(t_1-t_2)dt_2dt_1 \qquad (50)\\
&= 2T_0^2\Big[\Theta_{P_2}(\omega_2T_0)-\Theta_{P_2}(\omega_1T_0)\Big],
\end{aligned}
$$

where the function

$$
\Theta_{P_2}(y)=\lim_{x\to 0}\Theta_{P_1}(x,y)=\frac{1}{2}\left[\mathrm{Ei}(-y)+\frac{1-e^{-y}}{y^2}-\frac{2-e^{-y}}{y}\right], \qquad (51)
$$

and

$$
\begin{aligned}
P_3 = P_4 &= \int_0^{T_1}\int_{T_1}^{T_0+T_1}\tilde{\mathcal{T}}(t_2-t_1)\exp\left(-u_p(T_1-t_1)\right)dt_2dt_1 \qquad (52)\\
&= \frac{1}{u_p^2}\Big[\Theta_{P_3}(\omega_2|u_p,T_0,T_1)-\Theta_{P_3}(\omega_1|u_p,T_0,T_1)\Big], \quad \text{where}\\
\Theta_{P_3}(\omega|u_p,T_0,T_1) &= \mathrm{Ei}\left(-\omega T_0\right)\left(1+u_pT_0\right)-\mathrm{Ei}\left(-T_1\left(\omega+u_p\right)\right) \qquad (53)\\
&+ e^{-u_pT_1}\left[\mathrm{Ei}\left(-\omega T_1\right)\left(1+u_pT_1\right)-\mathrm{Ei}\left(-\omega\left(T_0+T_1\right)\right)\left(1+u_p(T_0+T_1)\right)\right]\\
&- e^{u_pT_0}\left[\mathrm{Ei}\left(-T_0\left(\omega+u_p\right)\right)-\mathrm{Ei}\left(-\left(T_0+T_1\right)\left(\omega+u_p\right)\right)\right]\\
&- \frac{u_p}{\omega}\left(1-e^{-\omega T_0}\right)\left(1-e^{-T_1(\omega+u_p)}\right)-\ln\left(\frac{\omega}{\omega+u_p}\right).
\end{aligned}
$$

In spite of cumbersome appearance, all integrals here have the same general form, with $P_j \propto \Theta_{P_j}(\omega_2\dots)-\Theta_{P_j}(\omega_1\dots)$ because the time correlation function Eq. (45) is a difference of two almost identical terms, differing only by substitution $\omega_2$ instead of $\omega_1$.

The cross-correlation terms are presented below only for the case of short delay, when $T_0 < T_1$. When evaluating these terms, we take into account that the shuttling velocity is not pathologically large or small, such that $\omega_1 \ll u_p \equiv \kappa_x v \ll \omega_2$. It is very important to notice that conditions like $\omega_1 < u_p < \omega_2$ and $0 < T_0 < T_1$ must be specified explicitly, in order to correctly treat the branching of the exponential integral function $\mathrm{Ei}(x)$ at zero and

choose the correct branch. The results are as follows.

$$C_1'' = \int_{T_1}^{T_0+T_1}\int_0^{T_0} \tilde{\mathcal{T}}(t_1-t_2)e^{-u_pT_1}dt_2dt_1 = e^{-u_pT_1}[\Theta_{c1}(\omega_2,T_0,T_1)-\Theta_{c1}(\omega_1,T_0,T_1)], \quad (54)$$

$$\Theta_{c1}(\omega,T_0,T_1) = g(\omega,T_1) - \frac{1}{2}\Big[g(\omega,T_1+T_0)+g(\omega,T_1-T_0)\Big], \quad (55)$$

$$g(\omega,T) = \frac{e^{-\omega T}(1-\omega T)}{\omega^2} - T^2\mathrm{Ei}(-\omega T),$$

$$C_2'' = C_4'' = \int_0^{T_1}\int_0^{T_0}\tilde{\mathcal{T}}(|t_2-t_1|)\exp\left(-u_pt_1\right)dt_2dt_1 \quad (56)$$

$$= \frac{1}{u_p^2}\Big[\Theta_{c2}(\omega_2|u_p,T_0,T_1)-\Theta_{c2}(\omega_1|u_p,T_0,T_1)\Big],$$

$$\Theta_{c2}(\omega|u_p,T_0,T_1) = \mathrm{Ei}(-\omega T_0)(u_pT_0-1)+\mathrm{Ei}\left[-T_1\left(\omega+u_p\right)\right] \quad (57)$$

$$+ e^{-u_pT_1}\left[\mathrm{Ei}(-\omega(T_1-T_0))\left(1+u_p\left(T_1-T_0\right)\right)-\mathrm{Ei}(-\omega T_1)\left(u_pT_1+1\right)\right]$$

$$+ e^{-u_pT_0}\left[\mathrm{Ei}\left[T_0\left(u_p-\omega\right)\right]-\mathrm{Ei}\left[-\left(T_1-T_0\right)\left(\omega+u_p\right)\right]\right]$$

$$+ \frac{u_p}{\omega}\left(1-e^{-T_0\omega}\right)\left(1-e^{-u_pT_1-\omega(T_1-T_0)}\right)$$

$$+ e^{-T_0u_p}\ln\left(\frac{T_1\left(\omega+u_p\right)}{|\omega-u_p|}\right)+\ln\left(\frac{\omega}{\omega+u_p}\right),$$

$$C_3'' = \int_0^{T_1}\int_{T_0}^{T_0+T_1}\tilde{\mathcal{T}}(|t_2-t_1|)\exp\left(-u_p|t_1-t_2+T_0|\right)dt_2dt_1 \quad (58)$$

$$= \frac{1}{u_p^2}\Big[\Theta_{c3}(\omega_2|u_p,T_0,T_1)-\Theta_{c3}(\omega_1|u_p,T_0,T_1)\Big],$$

$$\Theta_{c3}(\omega|u_p,T_0,T_1) = e^{-T_0u_p}\left[\left(u_p\left(T_1-T_0\right)-1\right)\ln\left(\frac{|\omega-u_p|}{\omega+u_p}\right)\right] \quad (59)$$

$$+ e^{-T_0u_p}\left(1-(T_1-T_0)u_p\right)\Big[\mathrm{Ei}\left(T_0\left(u_p-\omega\right)\right)-\mathrm{Ei}\left(-(T_1-T_0)\left(\omega+u_p\right)\right)\Big]$$

$$+ e^{T_0u_p}\left(1-\left(T_0+T_1\right)u_p\right)\Big[\mathrm{Ei}\left(-T_0\left(\omega+u_p\right)\right)-\mathrm{Ei}\left(-\left(\left(T_0+T_1\right)\left(\omega+u_p\right)\right)\right)\Big]$$

$$+ e^{-T_1u_p}\left(\mathrm{Ei}\left(-\omega(T_1-T_0)\right)+\mathrm{Ei}\left(-\omega\left(T_0+T_1\right)\right)\right)+2\left(T_1u_p-1\right)\mathrm{Ei}\left(-\omega T_0\right)$$

$$+ \frac{u_p\left(e^{-\omega T_0}-e^{-T_0u_p}\right)}{\omega-u_p}+\frac{u_p}{\omega+u_p}\Big[2e^{-T_1(\omega+u_p)}\cosh\left(T_0\omega\right)-e^{-\omega T_0}-e^{-T_0u_p}\Big].$$

Assembling all terms together, we obtain the dephasing factor for two entangled spins, forming an ST qubit, shuttled through pink sheet

$$\chi_{2,\mathrm{p}} = \frac{\sigma_{\mathrm{B}}^2}{\Delta}\left[\sum_{j=1}^{4}P_j - \sum_{j=1}^{4}C_j''\right], \quad (60)$$

In comparison with the case of OU sheet, see Eq. (39), the factor $\kappa_t^{-2}$ is removed due to the lack of a single characteristic time scale in the $1/f$ noise, such that the quantities $P_k$ and $C_k$ formally have the dimension of squared time.

## B. Asymptotic expansion

As discussed above, the physically relevant regime of $1/f$ noise corresponds to the situation where $\omega_1 \to 0$ and $\omega_2 \to \infty$. Therefore, we perform asymptotic expansions with respect to the cutoff frequencies and retain only the leading-order terms; since the integrals share the same form $C_k \propto \Theta_{c_k}(\omega_2) - \Theta_{c_k}(\omega_1)$, the two expansions can be performed independently, without ill-defined terms like $\omega_1 \cdot \omega_2$.

The function $\mathrm{Ei}(-x)$ in the limit $x \to +\infty$ has the form

$$\mathrm{Ei}(-x) = e^{-x}\left[-\frac{1}{x} + \frac{1}{x^2} + \mathcal{O}\big(x^{-3}\big)\right] \text{ at } x \to +\infty, \tag{61}$$

while for $x \to +0$,

$$\mathrm{Ei}(\pm x) = \gamma_E + \ln x \pm x + \frac{x^2}{4} + \mathcal{O}\big(x^3\big) \text{ at } x \to +0, \tag{62}$$

where $\gamma_E$ is Euler's constant. As a result, in the limit $\omega_2 \to +\infty$ and $\omega_1 \to +0$, the integrals $P_1$—$P_4$ and $C_1''$—$C_4''$ will retain the logarithmic corrections explicitly depending on $\omega_1$. Such corrections are a well-known feature of $1/f$ noise, which is often dominated by the low-frequency cutoff $\omega_1$ [31, 33–35]. The asymptotic form of each part is shown below.

$$P_1 \approx \frac{2}{u_p^2}\Big\{1 - (\gamma - 1)[\ln(\delta) + \mathrm{Ei}(-\gamma)] - e^{-\gamma}\left(1 + \gamma_E + \ln(\gamma\,\delta)\right)\Big\} \tag{63}$$

$$P_2 \approx \frac{\tau_p^2}{u_p^2}\left[\frac{3}{2} - \gamma_E - \ln\left(\tau_p\,\delta\right)\right] \tag{64}$$

$$\begin{aligned} P_3 \approx \frac{1}{u_p^2}\Big\{&\mathrm{Ei}(-\gamma) - e^{\tau_p}\left(\mathrm{Ei}\left(-\gamma - \tau_p\right) - \mathrm{Ei}\left(-\tau_p\right)\right) - e^{-\gamma}(\gamma + 1)\ln\left(\frac{\gamma}{\gamma + \tau_p}\right) \\ &- \gamma_E - \ln\left(\tau_p\right) - \tau_p\left[\left(\gamma_E - 1\right)\left(1 - e^{-\gamma}\right) + \ln\left(\tau_p\,\delta\right) - e^{-\gamma}\ln\left(\delta\left(\gamma + \tau_p\right)\right)\right]\Big\} \end{aligned} \tag{65}$$

$$C_1'' \approx \frac{e^{-\gamma}}{u_p^2}\left\{\gamma^2\ln\gamma + \tau_p\gamma\ln\left(\frac{\gamma - \tau_p}{\gamma + \tau_p}\right) + \tau_p^2\left(\frac{3}{2} - \ln\delta - \gamma_E\right) - \frac{\gamma^2 + \tau_p^2}{2}\ln\left(\gamma^2 - \tau_p^2\right)\right\} \tag{66}$$

$$\begin{aligned} C_2'' \approx \frac{1}{u_p^2}\Big\{&e^{-\tau_p}[\mathrm{Ei}\left(\tau_p - \gamma\right) - \mathrm{Ei}\left(\tau_p\right)] + e^{-\gamma}(\gamma + 1)\ln\left(\frac{\gamma}{\gamma - \tau_p}\right) \\ &+ \tau_p\left[e^{-\gamma}\ln\left(\delta\left(\gamma - \tau_p\right)\right) - \ln(\tau_p\,\delta) - (1 - e^{-\gamma})(\gamma_E - 1)\right] + \ln\left(\tau_p\right) + \gamma_E - \mathrm{Ei}(-\gamma)\Big\} \end{aligned} \tag{67}$$

$$\begin{aligned} C_3'' \approx \frac{1}{u_p^2}\Big\{&2 - 2(\gamma - 1)[\ln(\tau_p\,\delta) + \gamma_E] - e^{-\gamma}\left(2(1 + \gamma_E + \ln\delta) + \ln\big(\gamma^2 - \tau_p^2\big)\right) \\ &+ e^{-\tau_p}\left(\gamma - 1 - \tau_p\right)[\mathrm{Ei}(\tau_p) - \mathrm{Ei}(\tau_p - \gamma)] + e^{\tau_p}\left(\gamma - 1 + \tau_p\right)\left(\mathrm{Ei}\left(-\tau_p\right) - \mathrm{Ei}\left(-\gamma - \tau_p\right)\right)\Big\} \end{aligned} \tag{68}$$

Here we use dimensionless quantities $\gamma \equiv \kappa_x L = u_p T_1$, $\tau_p = u_p T_0$ and $\delta = \omega_1/u_p$. Assembling all terms in Eq. (60), we obtain the asymptotic expression for the dephasing factor at $\omega_1 \to 0$, $\omega_2 \to \infty$:

$$\chi_{2,\mathrm{p}} \approx \frac{\sigma_B^2}{\Delta u_p^2}\Big\{\tau_p^2\left[\frac{3}{2}-\gamma_E-\ln(\tau_p\,\delta)+e^{-\gamma}\left(\gamma_E+\frac{1}{2}\ln\left(\gamma^2-\tau_p^2\right)+\ln\delta-\frac{3}{2}\right)\right] \tag{69}$$
$$+2(\gamma-3)(\gamma_E+\ln\tau_p-\mathrm{Ei}(-\gamma))+\frac{e^{-\gamma}}{2}(\gamma^2+4\gamma+6)\ln\left(1-\frac{\tau_p^2}{\gamma^2}\right)-e^{-\gamma}(\gamma+2)\tau_p\ln\left(\frac{\gamma-\tau_p}{\gamma+\tau_p}\right)$$
$$+e^{-\tau_p}\left(-\gamma+\tau_p+3\right)\left[\mathrm{Ei}\left(\tau_p\right)-\mathrm{Ei}\left(\tau_p-\gamma\right)\right]-e^{\tau_p}\left(\gamma+\tau_p-3\right)\left[\mathrm{Ei}\left(-\tau_p\right)-\mathrm{Ei}\left(-\gamma-\tau_p\right)\right]\Big\}$$

Eq. (69) can be further simplified in the regime of large shuttling distances, $\gamma \sim 20-100 \gg 1$, and short delays $\tau_p$, when $e^{-\gamma} \to 0$ and $\mathrm{Ei}(-\gamma \pm \tau_p) \to 0$:

$$\chi_{2,\mathrm{p}} \approx \frac{\sigma_B^2}{\Delta u_p^2} \times \tag{70}$$
$$\left\{\tau_p^2\left[\frac{3}{2}-\gamma_E-\ln(\tau_p\,\delta)\right]+2(\gamma-3)\left(\gamma_E+\ln\tau_p\right)-e^{\tau_p}(\gamma+\tau_p-3)\mathrm{Ei}(-\tau_p)-e^{-\tau_p}(\gamma-\tau_p-3)\mathrm{Ei}(\tau_p)\right\}$$

Expanding this expression at small $\tau_p$ up to the second order, we obtain the result presented in the main text, in the limit $\gamma \gg 1$ and $\tau_p \ll 1$.

---


[1] B. I. Shklovskii and A. L. Efros, *Electronic properties of doped semiconductors*, Springer Series in Solid-State Sciences, Vol. 45 (Springer, Berlin, 1984).

[2] A. Abragam and B. Bleaney, *Electron paramagnetic resonance of transition ions* (Oxford University Press, Oxford, 2012).

[3] C. P. Slichter, *Principles of Magnetic Resonance*, 3rd ed. (Springer-Verlag, Berlin; Heidelberg; New York, 1996).

[4] V. Langrock, J. A. Krzywda, N. Focke, I. Seidler, L. R. Schreiber, and L. Cywiński, Blueprint of a scalable spin qubit shuttle device for coherent mid-range qubit transfer in disordered Si/SiGe/$SiO_2$, PRX Quantum **4**, 020305 (2023).

[5] M. Jeon, S. C. Benjamin, and A. J. Fisher, Robustness of electron charge shuttling: Architectures, pulses, charge defects and noise thresholds (2024), arXiv:2408.03315 [cond-mat.mes-hall].

[6] S. Bosco, J. Zou, and D. Loss, High-fidelity spin qubit shuttling via large spin-orbit interactions, PRX Quantum **5**, 020353 (2024).

[7] T. Struck, M. Volmer, L. Visser, T. Offermann, R. Xue, J.-S. Tu, S. Trellenkamp, Ł. Cywiński, H. Bluhm, and L. R. Schreiber, Spin-EPR-pair separation by conveyor-mode single electron shuttling in Si/SiGe, Nature Communications **15**, 1325 (2024).

[8] M. Volmer, T. Struck, A. Sala, B. Chen, M. Oberländer, T. Offermann, R. Xue, L. Visser, J.-S. Tu, S. Trellenkamp, Ł. Cywiński, H. Bluhm, and L. R. Schreiber, Mapping of valley-splitting by conveyor-mode spin-coherent electron shuttling, npj Quantum Inf. **10**, 61 (2024).

[9] D. A. Lidar, I. L. Chuang, and K. B. Whaley, Decoherence-free subspaces for quantum computation, Phys. Rev. Lett. **81**, 2594 (1998).

[10] P. Zanardi and M. Rasetti, Noiseless quantum codes, Phys. Rev. Lett. **79**, 3306 (1997).

[11] L. Viola, E. M. Fortunato, M. A. Pravia, E. Knill, R. Laflamme, and D. G. Cory, Experimental realization of noiseless subsystems for quantum information processing, Science **293**, 2059 (2001).

[12] B. Jadot, P.-A. Mortemousque, E. Chanrion, V. Thiney, A. Ludwig, A. D. Wieck, M. Urdampilleta, C. Bäuerle, and T. Meunier, Distant spin entanglement via fast and coherent electron shuttling, Nat. Nanotechnol. **16**, 570 (2021).

[13] N. Chentsov, Wiener random fields depending on several parameters, Doklady Akademii Nauk SSSR **106**, 607 (1956).

[14] T. Kitagava, Analysis of variance applied to function spaces, Memoirs of the Faculty of Science, Kyushu University Series A **6**, 41 (1951).

[15] R. J. Adler, *The geometry of random fields* (John Wiley & Sons Inc, Chichester, 1981).

[16] A. S. Mokeev, Y.-N. Zhang, and V. V. Dobrovitski, Modeling of decoherence and fidelity enhancement during transport of entangled qubits (2024), arXiv:2409.04404.

[17] J. S. Rojas-Arias, A. Noiri, P. Stano, T. Nakajima, J. Yoneda, K. Takeda, T. Kobayashi, A. Sammak, G. Scappucci, D. Loss, and S. Tarucha, Spatial noise correlations beyond nearest neighbors in $^{28}$Si/Si-Ge spin qubits, Phys. Rev. Appl. **20**, 054024 (2023).

[18] J. Zou, S. Bosco, and D. Loss, Spatially correlated classical and quantum noise in driven qubits: The good, the bad, and the ugly (2023).

[19] J. Yoneda, J. S. Rojas-Arias, P. Stano, K. Takeda, A. Noiri, T. Nakajima, D. Loss, and S. Tarucha, Noise-correlation spectrum for a pair of spin qubits in silicon, Nat. Phys. **19**, 1793 (2023).

[20] T. Struck, A. Hollmann, F. Schauer, O. Fedorets, A. Schmidbauer, K. Sawano, H. Riemann,

N. V. Abrosimov, Ł. Cywiński, D. Bougeard, and L. R. Schreiber, Low-frequency spin qubit energy splitting noise in highly purified $^{28}$Si/SiGe, npj Quantum Inf. **6**, 40 (2020).

[21] L. Cywiński, W. M. Witzel, and S. Das Sarma, Pure quantum dephasing of a solid-state electron spin qubit in a large nuclear spin bath coupled by long-range hyperfine-mediated interactions, Phys. Rev. B **79**, 245314 (2009).

[22] V. V. Dobrovitski, A. E. Feiguin, R. Hanson, and D. D. Awschalom, Decay of Rabi oscillations by dipolar-coupled dynamical spin environments, Phys. Rev. Lett. **102**, 237601 (2009).

[23] Wolfram Research, Inc., Mathematica, Version 13.3, Champaign, IL, 2024.

[24] M. Kepa, Ł. Cywiński, and J. A. Krzywda, Correlations of spin splitting and orbital fluctuations due to 1/f charge noise in the Si/SiGe quantum dot, Applied Physics Letters **123**, 034003 (2023).

[25] B. Shalak, C. Delerue, and Y.-M. Niquet, Modeling of spin decoherence in a Si hole qubit perturbed by a single charge fluctuator, Phys. Rev. B **107**, 125415 (2023).

[26] C. Spence, B. Cardoso-Paz, V. Michal, E. Chanrion, D. J. Niegemann, B. Jadot, P.-A. Mortemousque, B. Klemt, V. Thiney, B. Bertrand, L. Hutin, C. Bäuerle, F. Balestro, M. Vinet, Y.-M. Niquet, T. Meunier, and M. Urdampilleta, Probing charge noise in few electron CMOS quantum dots (2022), arXiv:2209.01853 [cond-mat.mes-hall].

[27] M. M. E. K. Shehata, G. Simion, R. Li, F. A. Mohiyaddin, D. Wan, M. Mongillo, B. Govoreanu, I. Radu, K. De Greve, and P. Van Dorpe, Modeling semiconductor spin qubits and their charge noise environment for quantum gate fidelity estimation, Phys. Rev. B **108**, 045305 (2023).

[28] G. Burkard, T. D. Ladd, A. Pan, J. M. Nichol, and J. R. Petta, Semiconductor spin qubits, Rev. Mod. Phys. **95**, 025003 (2023).

[29] E. J. Connors, J. J. Nelson, L. F. Edge, and J. M. Nichol, Charge-noise spectroscopy of Si/SiGe quantum dots via dynamically-decoupled exchange oscillations, Nat. Commun. **13**, 940 (2022).

[30] F. Ye, A. Ellaboudy, D. Albrecht, R. Vudatha, N. T. Jacobson, and J. M. Nichol, Characterization of individual charge fluctuators in Si/SiGe quantum dots (2024), arXiv:2401.14541 [cond-mat.mes-hall].

[31] E. Paladino, Y. M. Galperin, G. Falci, and B. L. Altshuler, $1/f$ noise: Implications for solid-state quantum information, Rev. Mod. Phys. **86**, 361 (2014).

[32] P. Dutta and P. M. Horn, Low-frequency fluctuations in solids: $1/f$ noise, Rev. Mod. Phys.

**53**, 497 (1981).

[33] M. Mehmandoost and V. V. Dobrovitski, Decoherence induced by a sparse bath of two-level fluctuators: Peculiar features of $1/f$ noise in high-quality qubits, Physical Review Research **6**, 033175 (2024).

[34] L. Cywiński, R. M. Lutchyn, C. P. Nave, and S. Das Sarma, How to enhance dephasing time in superconducting qubits, Phys. Rev. B **77**, 174509 (2008).

[35] J. Schriefl, Y. Makhlin, A. Shnirman, and G. Schön, Decoherence from ensembles of two-level fluctuators, New Journal of Physics **8**, 1 (2006).
